# Supplementary material for: Intermittent thermal convection in jammed emulsions
Source: arXiv:2405.02135 ancillary file (2024-12-17)
Supplement: Supplementary file 1 [file supplementary_material.pdf]

# <u>SUPPLEMENTARY MATERIAL FOR</u>: Intermittent Thermal Convection in Jammed Emulsions

Francesca Pelusi,[1,*] Andrea Scagliarini,[2,3] Mauro Sbragaglia,[4] Massimo Bernaschi,[2] and Roberto Benzi[4]

[1] *Istituto per le Applicazioni del Calcolo, CNR - Via Pietro Castellino 111, 80131 Naples, Italy*
[2] *Istituto per le Applicazioni del Calcolo, CNR - Via dei Taurini 19, 00185 Rome, Italy*
[3] *INFN, Sezione Roma "Tor Vergata", Via della Ricerca Scientifica 1, 00133 Rome, Italy*
[4] *Department of Physics & INFN, Tor Vergata University of Rome, Via della Ricerca Scientifica 1, 00133 Rome, Italy*

## I. METHODOLOGICAL DETAILS

*Hydrodynamical Equations:* In this work, we employed the open-source TLBfind code [1], which has been extensively validated and used in simulating thermal convection in emulsions systems [2, 3]. This code is based on a multi-component diffuse-interface lattice Boltzmann model [4–6], and evolves numerically the incompressible Navier-Stokes equations for the velocity field $\boldsymbol{u}(x, z, t)$ in a two-dimensional domain. The Navier-Stokes equations are coupled with an advection-diffusion equation for the temperature field $T(x, z, t)$ with a thermal diffusivity $\kappa$; the back-reaction of the temperature field in the Navier-Stokes equations is set through a buoyancy term in the Boussinesq approximation [7]. The resulting equations read (repeated indexes are summed upon):

$$\rho \left(\partial_t + u_k \partial_k\right) u_i = -\partial_j P_{ij} + \partial_j [\eta \left(\partial_i u_j + \partial_j u_i\right)] + \rho\, \alpha\, g\, T\, \delta_{iz} \ , \tag{1}$$

$$\partial_t T + u_i \partial_i T = \kappa \partial_{ii} T \qquad i = x, z \ , \tag{2}$$

where $\rho$ is the emulsion density, $\eta = \rho\nu$ is the bulk viscosity (with $\nu$ being the kinematc viscosity), $P_{ij}$ is the non-ideal pressure tensor responsible for the physico-chemical properties of the emulsion droplets, $\alpha$ is the thermal expansion coefficient, and $g$ is the strength of gravity acceleration. A disjoining pressure is introduced at the interface between the emulsion droplets [8–10] (to inhibit droplets' coalescence) and interactions between the droplets and the walls are tuned in such a way that droplets weakly adhere to the walls.
Notice that TLBfind [1] can simulate suspensions of droplets with non-ideal interfaces and non-zero surface tensions, but it is not suitable, in its present form, for other systems such as micro-gel suspensions. However, numerical strategies could extend the lattice Boltzmann methodology to support the modeling of micro-gel suspensions and the simulation of concentrated suspensions of elastic membranes with specific elastic properties. For instance, an extended code, coupling the lattice Boltzmann with the Immersed Boundary Method, could be used for that purpose, as demonstrated in several studies [11–15].

*System setup:* In this work, we simulate a jammed emulsion (volume fraction of the initially dispersed phase $\phi = 80\%$) consisting of two immiscible equiviscous fluids in the Rayleigh-Bénard setup, where the emulsion is confined between two parallel no-slip walls at $z = \pm H/2$ kept at the temperatures $T(x, z = +H/2, t) = T_{\text{cold}} < T_{\text{hot}} = T(x, z = -H/2, t)$ under the action of gravity in the direction of the thermal gradient (see Fig.1(a) of the main text) [16–18]. Periodic boundary conditions are applied in the $x$-direction. The domain size is set to $L \times H$ with $L \approx 2H$ and $H \approx 20d$, where $d$ is the average droplet diameter. Notice that the intermittent phenomenon discussed in the main text still persists in the case of a jammed emulsion placed in a domain with size ratio $\Gamma = L/H = 4$ (data not shown).

*System preparation:* The emulsion is initialized with a number $\text{N}_{\text{drops}} \approx 750$ of circular droplets whose centers of mass $\mathbf{X}_i$ ($i = 1...\text{N}_{\text{drops}}$) are first arranged in an honeycomb-like configuration and then a small stochastic displacement (ruled by a random seed) is added to the $\mathbf{X}_i$'s. After this initialization, the emulsion is further relaxed with no applied buoyancy, resulting in a slightly polydisperse emulsion [1] (see Fig.1(a) of the main text) and the resulting configuration exhibits a well defined yield stress (see Section II). The temperature field is initialized with a linear profile, $T(x, z, 0) = T_{\text{hot}} - \Delta T(z/H + 1/2)$, where $\Delta T = T_{\text{hot}} - T_{\text{cold}}$. After the emulsion preparation, we apply a perturbation to the hydrodynamical velocity to trigger the thermal convection. The shape of this perturbation is a combination

* francesca.pelusi@cnr.it

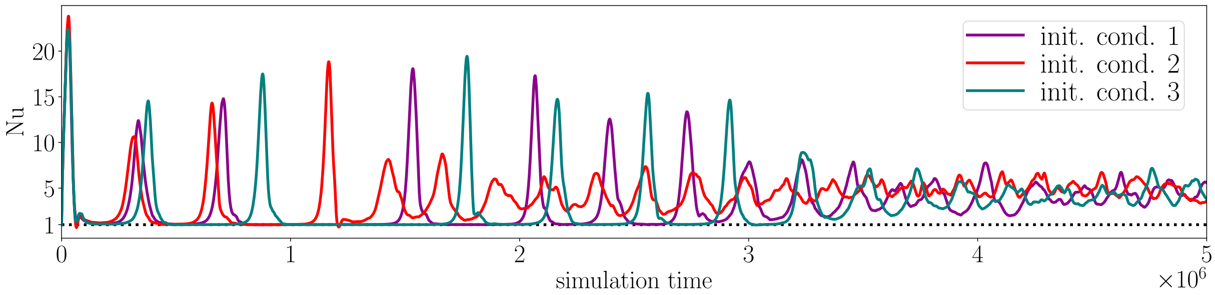


FIG. 1. Time evolution of the Nusselt number Nu for different random seeds in the initial condition. The first one (purple solid line) coincides with the one discussed and shown in Fig.1 of the main text. Simulation time is reported in lattice Boltzmann units.

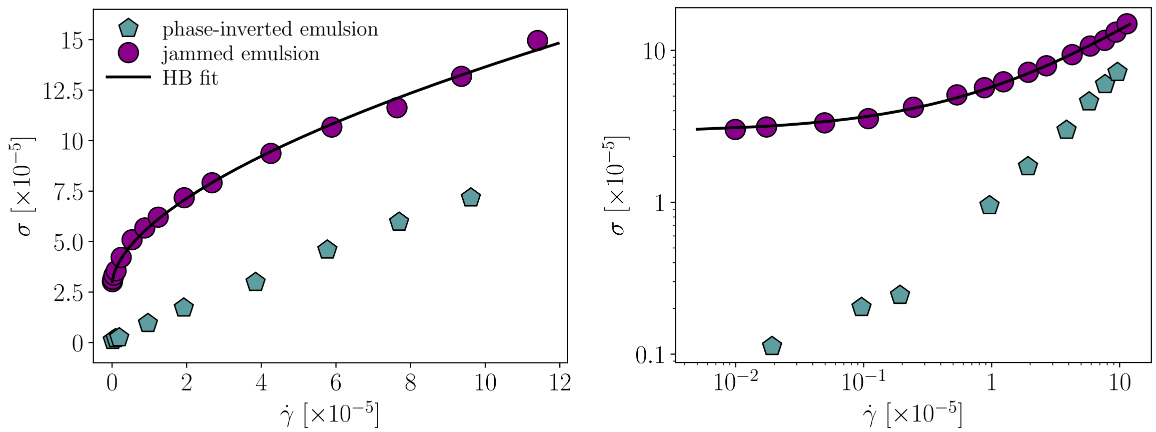


FIG. 2. Rheological flow-curves for the jammed emulsion (●, see also Fig.1(a) of the main text) and for the phase-inverted emulsion (⬟, see also Fig.1(e) of the main text), reporting the shear stress $\sigma$ as a function of the shear rate $\dot{\gamma}$. Left panel refer to the lin-lin representation, while on the right panel the same data are shown in log-log scale. Solid black lines refer to the fitting curve with Eq. (3) with $\sigma_0 = 2.89 \times 10^{-5}$, $A = 2.2 \times 10^{-2}$, and $n = 0.577$. Data and fitting parameters are expressed in lattice Boltzmann simulation units [1].

of sinusoidal functions along both directions with a small finite amplitude, which satisfies $\nabla \cdot \boldsymbol{u} = 0$. Different initial configurations can be obtained just changing the random seed in the initial preparation protocol. The impact of a different initial configuration on the time evolution of the Nusselt number (Nu) is shown in Fig. 1. Note that the simulation time shown in the figures reporting the time evolution of Nu is such that one free-fall time $t_{\mathrm{FF}} = \sqrt{H/\alpha g \Delta T}$ is $t_{\mathrm{FF}} \approx 10^4$ simulation time steps for the Rayleigh number of interest, $\mathrm{Ra} = \alpha g \Delta T H^3/(\kappa\nu) \approx 4 \times 10^5$.

## II. SYSTEM RHEOLOGY

We work in a Couette setup, where the emulsion is confined between two parallel flat walls with domain size $L \times H$, equal to the domain size used for thermal convection experiments. We move both walls with constant and opposite velocities along the $x$-direction $u_x(x, z = \pm H/2, t) = \pm u_w$ with no buoyancy activated. For each value of the imposed shear rate $\dot{\gamma} = 2u_w/H$, we measure the shear stress $\sigma$ that is an output of the simulation code [1]. We characterized the rheology of the jammed emulsion (see Fig.1(a) of the main text) and the phase inverted emulsion (see Fig.1(e) of the main text). Resulting data are shown in Fig. 2. For the rheological data of the jammed emulsion, we also report a fit with the Herschel–Bulkley (HB) law (solid black line)

$$\sigma = \sigma_0 + A\dot{\gamma}^n \ , \tag{3}$$

where $\sigma_0$ is the yield stress, $A$ is the consistency index and $n$ is the flux index. Fitting procedure results in the following values of HB parameters (expressed in lattice Boltzmann simulation units): $\sigma_0 = 2.89 \times 10^{-5}$, $A = 2.2 \times 10^{-2}$, and $n = 0.577$. Notice that, in our simulations, the surface tension is $\Sigma \approx 0.04$ and the average droplet radius is $R \approx 25$,

thus the yield stress value in units of the Laplace pressure is $\sigma_0/(\Sigma/R) \approx 1.5 \times 10^{-2}$. This value is comparable with experimental measurements in the same range of volume fractions ($\phi \sim 0.7 \div 0.8$) [19].

## III. ROLE OF THE YIELD STRESS

To investigate the role of the yield stress and verify whether the observed intermittency is due to the elastoplasticity of the emulsion rather than a two-phase flow effect, we conducted dedicated simulations at a fixed Ra $\approx 4 \times 10^5$, focusing on systems with vanishing yield stress. In a first numerical experiment, we compared the dynamics of the jammed emulsion ($\phi \sim 80\%$) with an emulsion prepared similarly but with the disjoining pressure (which stabilizes droplets against coalescence) switched off after the initial perturbation (see Section I). Signals of the Nusselt number Nu are reported in Fig. 3, with the solid purple line for $\phi \sim 80\%$ and the solid pink line for the case with disjoining pressure off. In the latter case, intermittency in the transient of Nu is lost. Selected density snapshots reveal droplet coalescence in favor of the inverted phases. This result confirms that a jammed state of stabilized finite-sized droplets (hence, elastoplasticity) is crucial for triggering intermittent heat bursts. In a second numerical experiment, we examined a moderately concentrated emulsion where droplets are stabilized against coalescence (i.e., disjoining pressure is active) but at a volume fraction where the rheology does not exhibit yield stress ($\phi \sim 60\%$, see Fig. 4(a)-(b)). Fig. 4(c) shows the comparison between the time evolution of Nu for the jammed emulsion ($\phi \sim 80\%$, solid purple line) and the one for $\phi \sim 60\%$ (solid blue line). This experiment further confirms that a two-phase state of stabilized droplets without yield stress is insufficient to trigger intermittent heat bursts.

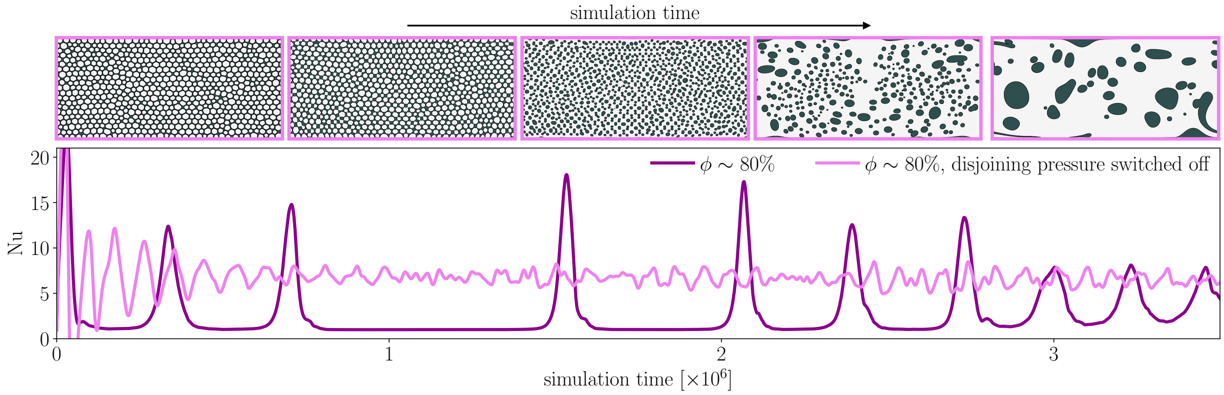


FIG. 3. Comparison of the time-evolution of the Nusselt number Nu at fixed fixed Ra $\approx 4 \times 10^5$ between the jammed emulsion ($\phi \sim 80\%$, purple solid line, the same signal as the one discussed and shown in Fig.1 of the main text) and a second one which has been prepared in the same way, but with disjoining pressure switched off (pink solid line). For the latter case, we also report some selected density snapshots during the evolution where droplet coalescence in favor of the inverted phases occurs.

## IV. RANGE OF RAYLEIGH NUMBER TRIGGERING INTERMITTENCY

To provide more quantitative details on the conditions triggering the intermittency described in the main text, we performed dedicated numerical simulations for the jammed emulsion at varying the Rayleigh number Ra. In Fig. 5, we report the time evolution of the Nusselt number Nu for different values of Ra (using different colors). The purple signal coincides with the one of the main text (Ra $\approx 4 \times 10^5$). These data confirm that the intermittency phenomenon is absent below a given threshold where the system is in a conductive state and convection is suppressed. This threshold value of Ra is around $\mathrm{Ra_{int}} \approx 3.25 \times 10^5$. Importantly, the intermittency appears in a finite rage of Ra between Ra $\approx 3.25 \times 10^5 \div 4.25 \times 10^5$ but at larger values of Ra a quicker transition to the convective state in the phase-inverted emulsion is prompted through more frequent coalescence events, characterized by a sequence of rigidity-fluidization transitions, thus bypassing the intermittent behavior.

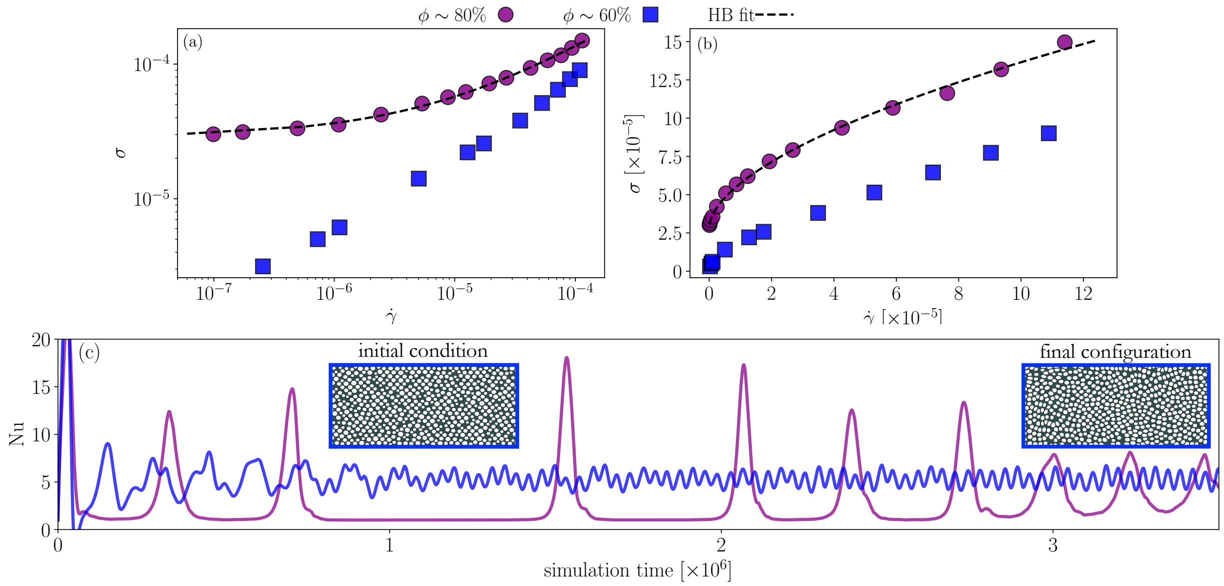


FIG. 4. Panels (a)-(b): Comparison of rheological flow-curves, relating shear stress $\sigma$ and shear rate $\dot{\gamma}$, between the jammed emulsion ($\phi \sim 80\%$, ●) and a second emulsion which does not present a value of the yield stress different from zero ($\phi \sim 60\%$, ■). Panel (a) refer to the log-log representation, whereas panel (b) refer to the lin-lin representation. Panel (c) shows the corresponding time-evolution of the Nusselt number Nu (colors match) at fixed fixed Ra $\approx 4 \times 10^5$, together with two density snapshots showing the initial condition and the final configuration for $\phi \sim 60\%$, respectively. Data for the jammed emulsion coincide with the ones discussed and shown in Fig.1 of the main text. Simulation time is reported in lattice Boltzmann units.

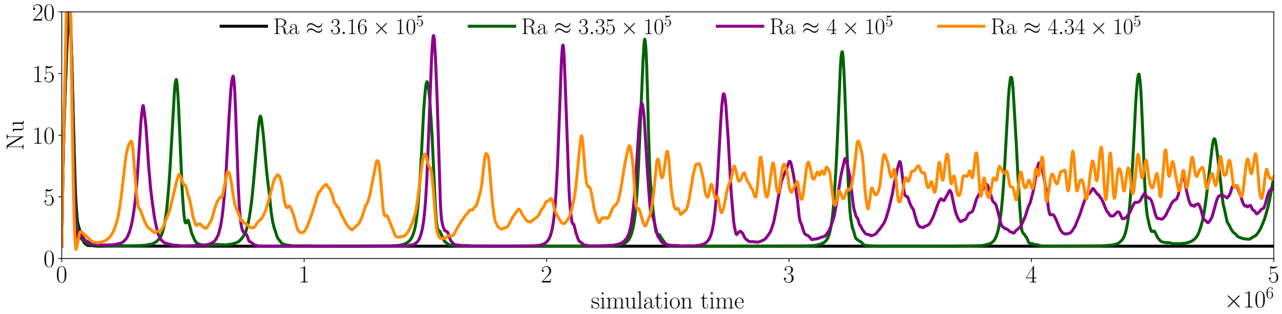


FIG. 5. Time evolution of the Nusselt number Nu for different values of the Rayleigh number Ra (different colors). Data for Ra $\approx 4 \times 10^5$ coincide with the ones discussed and shown in Fig.1 of the main text. Simulation time is reported in lattice Boltzmann units.

## V. DECOMPOSITION OF NUSSELT NUMBER INTO DROPLETS CONTRIBUTIONS

Fig. 6 provides evidence that Eq.(2) of the main text, giving a decomposition of the macroscopic Nusselt number Nu into the various contributions at the droplet scale $\mathrm{Nu}_i^{(\mathrm{drop})}$, holds. At any simulation time step and for each droplet, we measure $\mathrm{Nu}_i^{(\mathrm{drop})}$, with $i = 1 \ldots \mathrm{N}_{\mathrm{drops}}$, as described in the main text; then, we compute the average value (over all the droplets) at that time step as

$$\langle \mathrm{Nu}^{(\mathrm{drop})} \rangle_{\mathrm{N}_{\mathrm{drops}}} = \frac{1}{\mathrm{N}_{\mathrm{drops}}} \sum_{i=1}^{\mathrm{N}_{\mathrm{drops}}} \mathrm{Nu}_i^{(\mathrm{drop})} \tag{4}$$

and show the corresponding result in Fig. 6 (filled circles) together with the macroscopic Nusselt number Nu computed using Eq.(1) of the main text (solid purple line).

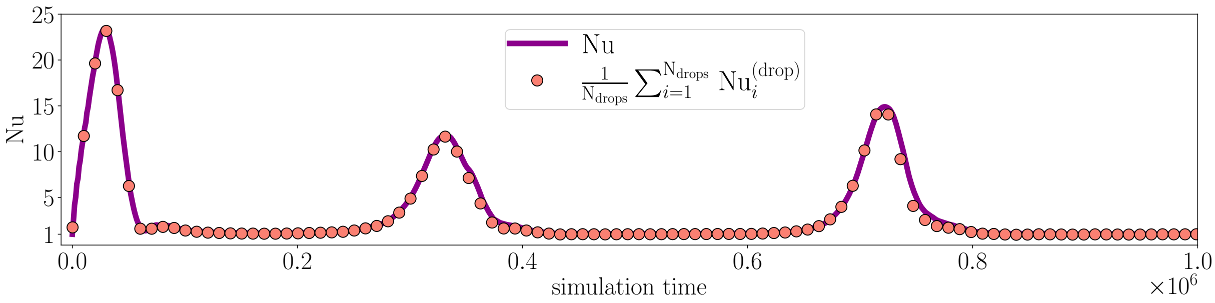


FIG. 6. Time evolution of the macroscopic Nusselt number Nu (solid purple line, from Eq.(1) of the main text) together with the average value of the droplet Nusselt number (●, see also Eq. (4)). Simulation time is reported in lattice Boltzmann units.

## VI. DETAILS ON THE CALCULATION OF THE CORRELATION FUNCTION C($r$)

The definition of C($r$) (Eq.(3) of the main text) is the result of a three-steps procedure: ($i$) we consider the time evolution of the Nusselt number Nu; ($ii$) each simulation time step $t$ is assigned a label depending on the regime the time $t$ belongs to, namely: a) heat burst, b) resting period, c) sustained convection; ($iii$) we compute the interface displacement $A_\tau(x_k, z_k, t)$ at any time $t$ and we associate the obtained value to the dataset corresponding to the label of $t$. Finally, we repeat these steps for tens of simulations corresponding to different initial configurations of the same emulsion (see Section I), thus collecting 3 datasets, one for each regime (i.e., a,b,c). For each dataset/regime, we compute C($r$), resulting in data reported in Fig.4 of the main text.

---


[1] F. Pelusi, M. Lulli, M. Sbragaglia and M. Bernaschi, *Computer Physics Communications*, 2022, **273**, 108259.
[2] F. Pelusi, M. Sbragaglia, R. Benzi, A. Scagliarini, M. Bernaschi and S. Succi, *Soft Matter*, 2021, **17**, 3709–3721.
[3] F. Pelusi, S. Ascione, M. Sbragaglia and M. Bernaschi, *Soft Matter*, 2023, **19**, 7192–7201.
[4] R. Benzi, S. Succi and M. Vergassola, *Physics Reports*, 1992, **222**, 145–197.
[5] T. Krüger, H. Kusumaatmaja, A. Kuzmin, O. Shardt, G. Silva and E. M. Viggen, *Springer International Publishing*, 2017, **10**, 4–15.
[6] S. Succi, *The lattice Boltzmann Equation*, Oxford University Press, 2018.
[7] D. Lohse and K.-Q. Xia, *Annual Review of Fluid Mechanics*, 2010, **42**, 335–364.
[8] R. Benzi, M. Sbragaglia, S. Succi, M. Bernaschi and S. Chibbaro, *J. Chem. Phys.*, 2009, **131**,.
[9] M. Sbragaglia, R. Benzi, M. Bernaschi and S. Succi, *Soft Matter*, 2012, **8**, 10773–10782.
[10] B. Dollet, A. Scagliarini and M. Sbragaglia, *J. Fluid Mech.*, 2015, **766**, 556–589.
[11] M. Gross, T. Krüger and F. Varnik, *Soft Matter*, 2014, **10**, 4360–4372.
[12] D.-K. Sun, Y. Wang, A.-P. Dong and B.-D. Sun, *International Journal of Heat and Mass Transfer*, 2016, **94**, 306–315.
[13] O. Aouane, A. Scagliarini and J. Harting, *Journal of Fluid Mechanics*, 2021, **911**, A11.
[14] M. Wouters, O. Aouane, M. Sega and J. Harting, *Philosophical Transactions of the Royal Society A*, 2021, **379**, 20200399.
[15] F. Guglietta, F. Pelusi, M. Sega, O. Aouane and J. Harting, *Journal of Fluid Mechanics*, 2023, **971**, A13.
[16] S. Grossmann and D. Lohse, *Physical Review Letters*, 2001, **86**, 3316.
[17] G. Ahlers, S. Grossmann and D. Lohse, *Reviews of Modern Physics*, 2009, **81**, 503.
[18] F. Chillà and J. Schumacher, *The European Physical Journal E*, 2012, **35**, 1–25.
[19] T. Mason, J. Bibette and D. Weitz, *Journal of colloid and interface science*, 1996, **179**, 439–448.
